# Supplementary material for: Efficient inference in occlusion-aware generative models of images
Source: arXiv:1511.06362 source file (2016-02-16)
Supplement: Supplementary file 1 [file appendix.tex]

\subsection*{Appendix: Notation}

\begin{tabular}{cc}
VAE & \\
ST-VAE & \\
CST-VAE & \\
$x$ & b \\
 $x_i$ & d \\
  $L_i$ & d \\
   $C_i$ & d \\
   $T_i$ & d \\
$z^C_i$ & d \\
$z^T_i$ & d \\
$f_C(\cdot; \theta_C)$ & d \\
$f_T(\cdot; \theta_T)$ & d \\
$f_enc(\cdot ;\phi)$ & d \\
$P(x | z^C, z^T; \theta)$ & d \\
$Q(z^C, z^T | x; \phi)$ & d 
\end{tabular}
